# Supplementary material for: Stochastic Bandits with Vector Losses: Minimizing $\ell^\infty$-Norm of Relative Losses
Source: arXiv:2010.08061 source file (2020-10-15)
Supplement: Supplementary file 1 [file app_cg.tex]

\section{Proof of Theorem~\ref{thm:cg}}\label{app:cg}

% To begin with, we first prove the following lemma.
% \begin{lemma}\label{lemma:concentration}
% For any given $k,l\in[K]$ with $k\neq l$, if for all $i\in \left\{1,2\right\}$, we have $\abs{\hloss{i}{j}- \loss{i}{j}}\leq \epsilon$ for $j\in\{k,l,\star_1,\star_2\}$, then we have
% \begin{align*}
% \abs{\hclstar{k}{l}-\clstar{k}{l}} \leq 2\epsilon,
% \end{align*}
% and therefore, $\forall i\in \{1,2\}$,
% \begin{align*}
% \abs{\hcloss{i}{k}{l}-\closs{i}{k}{l}} \leq 3\epsilon.
% \end{align*}
% \end{lemma}

% \begin{proof}
% We have
% \begin{align*}
% \hclstar{k}{l} &= \max_{i\in\{1,2\}}\min_{\alpha\in[0,1]} (\alpha \hlstar{i}{k}+(1-\alpha)\hlstar{i}{l})\leq \max_{i\in\{1,2\}}\min_{\alpha\in[0,1]} \left(\alpha (\lstar{i}{k}+2\epsilon) +(1-\alpha)(\lstar{i}{l}+2\epsilon)\right)\\
% &= \max_{i\in\{1,2\}}\min_{\alpha\in[0,1]} (\alpha \lstar{i}{k}+(1-\alpha)\lstar{i}{l})+2\epsilon = \clstar{k}{l}+2\epsilon.
% \end{align*}
% Similarly we have $\hclstar{k}{l}\geq \clstar{k}{l}-2\epsilon$. The second inequality is trivial by definition.
% \end{proof}

We first show that the empirical estimation is valid with high probability at each round. Specifically, we have the following lemma.

\begin{lemma}\label{lemma:conc}
Define the following event:
\begin{align*}
    E_{1,t}\triangleq \left\{\forall k\in[K],i\in [d]: \abs{\hloss{i}{k}- \loss{i}{k}}\leq \sqrt{\dfrac{2\log(t)}{N_{k}}} \right\},
\end{align*}
where $N_{k}$ denotes the number of pulls of arm $k$. This event will happen with probability at least $1- dK/t^2$, that is:
\begin{align*}
    \PP {E_{1,t}} \geq 1- \frac{dK}{t^2}
\end{align*}
\end{lemma}

\begin{proof}
This is the a direct application of the Hoeffding's Inequality with the union bound.
\end{proof}

With the Lemma above, we proceed to show that $\LCB(\blstar{}{})$ is a valid approximation for $\blstar{}{}$. Concretely, we have the following lemma.

\begin{lemma}
Assume $E_{1,t}$ holds, we have,
\begin{align*}
    \LCB_t(\blstar{}{})_{i,k} \le \lstar{i}{k} \le \LCB_t(\blstar{}{})_{i,k} + 2\sqrt{\frac{2\log(t)}{N_{t,k}}} +2 \sqrt{\frac{2\log(t)}{N}}.
\end{align*}
\end{lemma}
\begin{proof}
This is a easy deduction of Lemma~\ref{lemma:conc}.
\end{proof}
