# Supplementary material for: Stochastic Bandits with Vector Losses: Minimizing $\ell^\infty$-Norm of Relative Losses
Source: arXiv:2010.08061 source file (2020-10-15)
Supplement: Supplementary file 3 [file app_misc.tex]

\section{Miscellaneous}\label{app:misc}

\subsection{Explicit expression for the relative loss of a combinatorial arm}

For a given combinatorial arm $(k,l)$, we have explicitly the following 4 cases,
\begin{align*}
    \clstar{k}{l}=\begin{cases}
    \max_{i\in\{1,2\}}\lstar{i}{k} \qquad \text{if}~~\loss{1}{k}\leq \loss{1}{l}~\&~ \loss{2}{k}\leq \loss{2}{l}\,,\\
    \max_{i\in\{1,2\}}\lstar{t}{l} \qquad \text{if}~~\loss{1}{k}\geq \loss{1}{l}~\&~ \loss{2}{k}\geq \loss{2}{l}\footnotemark\,, \\
    \min_{j\in \{k,l\}}\max_{i\in\{1,2\}}\lstar{i}{j} \qquad \text{if}~~(\lstar{1}{k}-\lstar{2}{k})(\lstar{1}{l}-\lstar{2}{l}) >0\,,\\
    \dfrac{\lstar{1}{k}\lstar{2}{l}-\lstar{1}{l}\lstar{2}{k}}{\lstar{1}{k}+\lstar{2}{l}-\lstar{1}{l}-\lstar{2}{k}} \qquad \text{otherwise}\,,
    \end{cases}
\end{align*}
where the first three cases actually only depends on a single arm.\footnotetext{With two equalities not attained simultaneously.}
