# Supplementary material for: Stochastic Bandits with Vector Losses: Minimizing $\ell^\infty$-Norm of Relative Losses
Source: arXiv:2010.08061 source file (2020-10-15)
Supplement: Supplementary file 4 [file app_notations.tex]

%!TEX root = ../main.tex
\section{Notation}\label{app:notations}

We recall and resemble the important notation in this section.

\begin{table}[h]
	\centering
	\caption{Table of notation}
	\begin{tabular}{@{}l|l@{}}
		\toprule
		\thead{Notation} & \thead{Meaning} \\ \midrule
		$K$ & number of arms \\
        $\dist{i}{k}$ & the $i$-th loss distribution for the $k$-th arm \\
        $\loss{i}{k}$ & $\mathbb{E}[\dist{i}{k}]$ \\
        $\bloss{i}$ & the vector loss of arm $i$ \\
        $\star_i$ & the set of the arms with the least $i$-th loss \\
        $\bLoss{\cA}$ & the cumulative loss of algorithm $\cA$ \\
        $\Loss{i}{\cA}$ & the cumulative $i$-th loss of algorithm $\cA$ \\
        $\bomega^\star$ & the optimal weight of arm pulls \\
        $R_\cA(T)$ & regret \\
        $\lstar{i}{k}$ & the $i$-th loss relative to $\star_i$ \\
        $\clstar{k}{l}$ & the minimum relative loss of the combinatorial arm $(k,l)$ \\
        $\hclstar{k}{l}$ & the empirical minimum relative loss of the combinatorial arm $(k,l)$ \\
        $\hwlstar{\bomega}$ & the empirical loss of weight $\bomega$ relative to $\star$ \\
        $\hhwlstar{\bomega}$ & The empirical loss of weight $\bomega$ relative to $\hat{\star}$ \\
        $\Delta = \min_{i, \loss{i}{k}-\loss{i}{l}>0} \loss{i}{k}-\loss{i}{l}$ & the minimum positive loss gap between any two arms \\
		\bottomrule
	\end{tabular}
\end{table}
